# Supplementary material for: On Distribution Dependent Sub-Logarithmic Query Time of Learned Indexing
Source: arXiv:2306.10651 source file (2023-06-19)
Supplement: Supplementary file 1 [file appendix.tex]

The algorithm recursively proceeds unless it exits to perform a binary search. At the last level of recursion, the size of the array is 2. At every iteration the size of the array is reduced to $\sqrt{n \log\log n}$. For $n\geq 1$, $\log\log n\leq n^{\frac{1}{4}}$, so that the size of the array at the $i$-th recursions is at most $n^{(\frac{3}{4})^i}$, Setting $n^{(\frac{3}{4})^i}\leq2$, we get that $i\leq \frac{\log \log n-\log\log 2}{\log \frac{4}{3}}$. Let $B_i$ denote the event that the algorithm exits to perform binary search at the $i$-th iteration.  Since the size of the array at the $i$-th iteration is $n^{(\frac{3}{4})^i}$, the binary search takes $\log n^{(\frac{3}{4})^i}$. Thus, the expected number of comparisons is $\sum_{i=1}^{\log\log n} 1+ p(B_i,\Tilde{B_{i-1}}, .... \Tilde{B_1})\log n^{(\frac{3}{4})^i}$. Note that 

\begin{align}
p(B_i,\Tilde{B_{i-1}}, .... \Tilde{B_1})=p(B_i|\Tilde{B_{i-1}}, .... \Tilde{B_1})p(\Tilde{B_{i-1}}, .... \Tilde{B_1})\leq p(B_i|\Tilde{B_{i-1}}, .... \Tilde{B_1})
\end{align}

At each iteration of the algorithm, $F_\chi'$ is the CDF from which the items in $A$ are i.i.d sampled. Therefore, by DKW, 

$$
P(|nF_\chi(q)'-nF_n(q)|\geq \rho\sqrt{n})\leq 2e^{-2\rho^2}
$$

$nF_n(q)$ is the actual position of $q$ in $A$ and $nF_\chi(q)$ is the estimated position. DKW implies that with the stated probability the observed position in the array differs at most $\rho\sqrt{n}$ from the estimated position. That is, the event $|nF_\chi(q)-nF_n(q)|\geq \rho\sqrt{n}$ happens if and only if $B_i$ happens, so that their probabilities are the same, i.e.,

$$
p(B_i|\Tilde{B_{i-1}}, .... \Tilde{B_1})\leq 2e^{-2\rho^2}.
$$

Now substitute $\rho=\sqrt{\frac{1}{2}\log\log n}$ so that $e^{-2\rho^2}=\frac{1}{\log n}$, which implies $p(B_i|\Tilde{B_{i-1}})\times \log n^{\frac{1}{2^i}}=1$. 

Now consider the case that we have access to $\hat{f}^{i, j}$ for all $i$ and $j$, that approximates $F_\chi(x)'$ for the sub-array $A[i, j]$ with approximation error $\frac{\sqrt{\log\log (j-i)}}{\sqrt{j-i}}$, so that $|n\hat{f}-nF_{\chi}'|\leq \sqrt{n\log\log (n)}$. 

$$
|n\hat{f}^{i, j}(q)-nF_n(q)| \leq |nF_\chi(q)'-n\hat{f}^{i, j}(q)|+|nF_\chi(q)'-nF_n(q)|
$$

$$
|n\hat{f}^{i, j}(q)-nF_n(q)| \leq \sqrt{n\log\log (n)}+|nF_\chi(q)'-nF_n(q)|
$$

Therefore, $|nF_\chi(q)'-nF_n(q)|\leq \rho\sqrt{n}$ implies
$$
|n\hat{f}^{i, j}(q)-nF_n(q)| \leq 2\sqrt{n\log\log (n)}
$$
So that 

$P(|n\hat{f}^{i, j}(q)-nF_n(q)| \leq 2\sqrt{n\log\log (n)})\geq P(|nF_\chi(q)'-nF_n(q)|\leq \rho\sqrt{n})$

And therefore 

$P(|n\hat{f}^{i, j}(q)-nF_n(q)| \geq 2\sqrt{n\log\log (n)})\leq \frac{1}{\log n}$

Note that the size of the array at the $i$-th level of recursion is at most $16n^{(\frac{3}{4})^i}$, so that binary search takes at most $\log 16n^{(\frac{3}{4})^i}$.

\qed
